# Supplementary material for: Probing hundreds of individual quantum defects in polycrystalline and amorphous alumina
Source: arXiv:2107.04131 source file (2022-03-01)
Supplement: Supplementary file 1 [file Supp.pdf]

# Supplementary materials for "Probing hundreds of individual quantum defects in polycrystalline and amorphous alumina"

Chih-Chiao Hung
*Laboratory for Physical Sciences, 8050 Greenmead Drive, College Park, Maryland 20740, USA*
*Quantum Materials Center, University of Maryland, College Park, Maryland 20742, USA and*
*Department of Physics, University of Maryland, College Park, Maryland 20742, USA*

Liuqi Yu and Neda Foroozani
*Laboratory for Physical Sciences, 8050 Greenmead Drive, College Park, Maryland 20740, USA and*
*Quantum Materials Center, University of Maryland, College Park, Maryland 20742, USA*

Stefan Fritz and Dagmar Gerthsen
*Laboratory for Electron Microscopy, Karlsruhe Institute of Technology, Karlsruhe, 76131, Germany*

Kevin D. Osborn
*Laboratory for Physical Sciences, 8050 Greenmead Drive, College Park, Maryland 20740, USA*
*Quantum Materials Center, University of Maryland, College Park, Maryland 20742, USA and*
*Joint Quantum Institute, University of Maryland, College Park, MD 20742, USA*
(Dated: February 28, 2022)

## S-I. ADDITIONAL DC SWEEP SPECTROSCOPY ON ALUMINA TLS

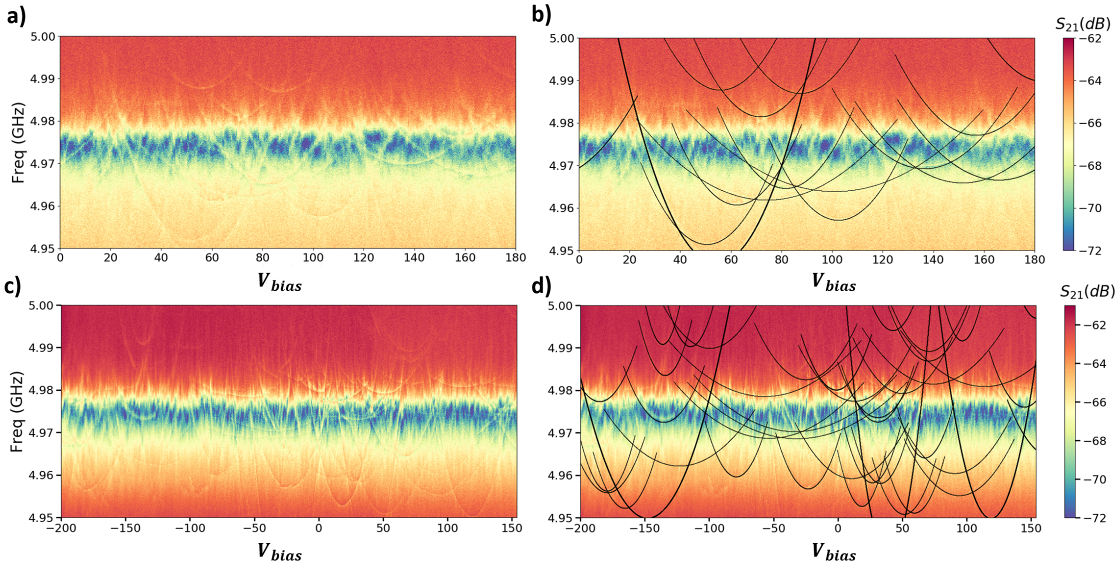


FIG. S1. TLS spectroscopy of $\gamma - \mathrm{Al_2O_3}$ TLS. Fig. (a) and (c) show two raw data sets, while Fig. (b) and (d) show TLS spectra with TLS fittings, respectively. The data sets are measured in different cooldowns.

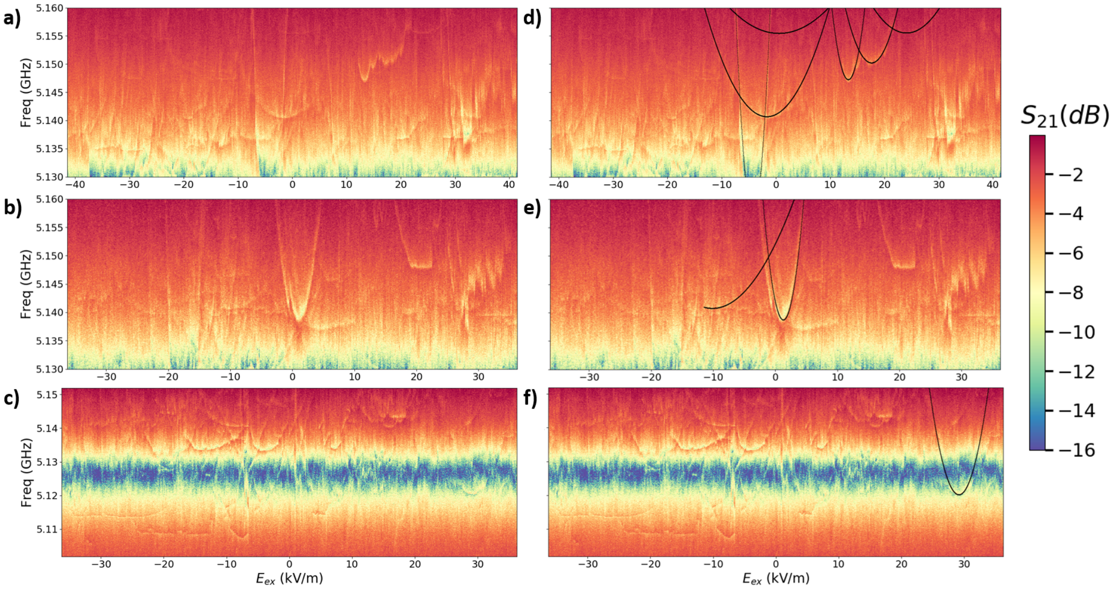


FIG. S2. TLS spectroscopy of $\mathrm{a - AlO_x}$. Fig (d), (e), (f) are the same data as (a), (b) and (c), respectively, with added fitting TLS traces. Three data sets are measured in different cooldowns.

In this section, we show spectroscopy data sets from different cooldowns on the two alumina types, which are not shown in the main text. Fig. S1 shows $\gamma - \mathrm{Al_2O_3}$ TLS spectra and Fig. S2 shows $a - \mathrm{AlO_x}$ TLS spectra in raw data. Note that sometimes there are only a couple of $a - \mathrm{AlO_x}$ TLSs extracted in the cooldown such as Fig. S2 (b) and (e).

Some interesting TLSs (those have asymmetric hyperbola or switch to unknown states) are shown in Fig. 3 in the main text. However, most of the fitted TLS traces show a minimum that is symmetric and fit to a hyperbola. We believe the asymmetric hyperbola is because of two TLSs with two dipole moment are closed in asymmetric energy such that one of the hyperbola is more obvious than the other one. The fit lines are showing the obvious one which cross their minimum energy.
